# Supplementary material for: Coulomb Enhanced Superconducting Pair Correlations in the Frustrated Quarter-Filled Band
Source: arXiv:1505.07496 ancillary file (2015-05-27)
Supplement: Supplementary file 1 [file supplemental-05-27-15.pdf]

# Supplementary Information: Coulomb Enhanced Superconducting Pair Correlations in the Frustrated Quarter-Filled Band

Niladri Gomes,[1] W. Wasanthi De Silva,[2] Tirthankar Dutta,[1] R. Torsten Clay,[2] and S. Mazumdar[1]

[1]*Department of Physics, University of Arizona, Tucson, AZ 85721*

[2]*Department of Physics and Astronomy and HPC*[2] *Center for Computational Sciences, Mississippi State, MS 39762*

(Dated: May 27, 2015)

## S.1. METHODS

*Exact diagonalization using the valence bond basis.* The valence bond (VB) method is a well known numerical technique for studying correlated quantum systems [S1][S2][S3]. In the present work it is used for computing pair-pair correlation functions and relative weights of nearest and next-nearest neighbour VB diagrams for the $4 \times 4$ lattice. The VB basis is complete and non-orthogonal. The main advantages of the the VB method are that it allows, first, visualization of wavefunctions in terms of the dominant VB diagrams, and second, conservation of total spin $S$. We have used this method to calculate correlation functions for the 4×4 lattice within the lowest $S = 0$ state for all values of $t_{x+y}$; for number of electrons 4, 8 and 12 the single-particle wavefunctions are degenerate, and for these cases calculations targeting specific total $S$ states would be difficult for methods conserving only $S_z$.

*PIRG.* The PIRG method was used to calculate zero-temperature expectation values of the pair-pair correlations. PIRG was used because conventional Monte Carlo methods (see below) are limited by the fermion sign problem to either small Hubbard $U$ and/or high temperatures for frustrated lattices. The PIRG method is described in Reference [S4]. Within PIRG, the wavefunction is expanded as a sum over $L$ Slater determinants, and the projector operator $\exp(-\tau H)$ is used to project out the ground state from a random starting determinant [S4]. The method is exact at $U = 0$ and for each $L$ PIRG calculations are variational. For the calculations presented here, we first minimized the variational energy for $L = 1$, followed by optimizing the variational state at $L = 8$. We then continued calculations to larger $L$, doubling ($L =$16, 32, …) $L$ at each step. We used a maximum $L$ of 512 for most results shown here. The finite basis bias is then removed by extrapolating quantities as a function of the energy variance ΔE [S4]. For the results presented here, we typically used a linear extrapolation in ΔE for the three largest $L$ used, i.e. $L$={128, 256, 512}.

Several additional techniques are essential to improve the accuracy of the PIRG. First, we incorporated lattice and spin symmetries using projection operators of the QP-PIRG method of Reference [S5]. The use of lattice and spin symmetries has been shown to drastically reduce the $L$ required to obtain accurate results with PIRG [S5]. Here we used the more accurate method of incorporating symmetries during projection (QP-PIRG) as opposed to afterwards (PIRG-QP) [S5]. For the lattice symmetry we used the full space group of the lattice (translations and point symmetries). For spin, we projected using the spin parity operator, which separates even and odd values of total spin $S$. All results here are for the even spin parity subspace. Second, it has been observed that in certain cases the PIRG method can be trapped in excited states [S6]. To help prevent this, in addition to the PIRG projection operator, we used a random simulated annealing-like modification of the Slater determinants [S6][S7]. Furthermore, several starting states were chosen for the projection, and their final energy compared.

PIRG has been extensively benchmarked against other methods. We previously compared the pair-pair correlations from PIRG and exact diagonalization on a 4×4 frustrated lattice and found essentially perfect agreement [S7]. For larger lattices, PIRG has further been checked against conventional quantum Monte Carlo for systems where there is no sign problem, such as the half-filled square lattice Hubbard model [S5]. Our comparisons of PIRG and DQMC (see Section S.3 below) further gives us confidence in the accuracy of the method.

*CPMC.* CPMC is a ground-state projector QMC method [S8]. Like PIRG, CPMC works in the space of Slater determinants. This space is overcomplete, which results in contributions to the ground state wavefunction that are both positive and negative. The Monte Carlo sampling is confined to the region where the overlap between each random walker $|\phi\rangle$ and a trial wavefunction $|\Psi_T\rangle$ is positive [S8]. This eliminates the loss of precision known as the fermion sign problem, but introduces an approximation into the method. The results presented here used the free-electron wavefunction for $|\Psi_T\rangle$. This trial function produces exact CPMC results at $U = 0$ and also for nonzero $U$ in the one-dimensional limit [S8]. While this choice has been shown to be accurate for many lattices, particularly for closed-shell fillings [S8], we restrict the use of CPMC to small $U$ ($0 < U \lesssim 2$). Our CPMC code results used an imaginary time discretization of $\Delta\tau = 0.1$ with a second-order Trotter approximation; the additional systematic error due to this approximation is negligible.

*DQMC.* The DQMC method integrates out the fermion degrees of freedom, replacing the Hubbard interaction with an auxiliary Hubbard-Stratonovich field [S9]; for a review see [S10]. Our results here used the finite-temperature variant of this algorithm.

This method suffers from sign problem when used for fermion systems. As shown in Fig. 3, in the 6×6 lattice an inverse temperature of at least $\beta \approx 8$ is required to see the enhancement of pairing at $\rho \simeq 0.5$. At these lower temperatures, the sign problem limits us to $U \approx 2$. Our results used a Trotter discretization in imaginary time of $\Delta\tau = 0.1$; for $U = 2$ the systematic error due to this approximation is smaller than the point size on our plots and can be neglected.

## S.2. CHOICE OF LATTICES

Our choice of which lattices to consider is guided by several considerations. First, the total number of sites should be less than around 100 in order to obtain accurate results for the pair-pair correlation functions. Second, the lattice should have a single-particle level structure such that quarter-filling ($\rho = 0.5$) is a non-degenerate state, and the $L_x$ and $L_y$ dimensions should be an even number of sites. We took $t_x$ slightly different from $t_y$ ($t_x = 1$, $t_y = 0.9$) in order to maximize the number of densities with non-degenerate single-particle spectra. Within these constraints, and considering only lattices for which $L_y \gtrsim L_x/2$, the only possible choices are 10×10, 10×6, 6×6. In addition we considered the 4×4 lattice, which although degenerate at $\rho = 0.5$, is the largest lattice for which the full density range can be calculated exactly.

## S.3. DISCUSSION OF DATA

The measure of SC we adopt is the equal-time pair-pair correlation function defined as $P_{ij} = \langle \Delta_i^\dagger \Delta_j \rangle$. The pair creation operator $\Delta_i^\dagger$ creating a pair on site $i$ is defined as

$$\Delta_i^\dagger = \sum_\nu g(\nu) \frac{1}{\sqrt{2}} (c_{i,\uparrow}^\dagger c_{i+\vec{r}_\nu,\downarrow}^\dagger - c_{i,\downarrow}^\dagger c_{i+\vec{r}_\nu,\uparrow}^\dagger). \tag{1}$$

The phases $g(\nu)$ determine the pairing symmetry. For $d_{x^2-y^2}$ symmetry, $g(\nu) = \{1,-1,1,-1\}$ for $\vec{r}_\nu = \{\hat{x},\hat{y},-\hat{x},-\hat{y}\}$ respectively. For $d_{xy}$ symmetry, $g(\nu) = \{1,-1,1,-1\}$ for $\vec{r}_\nu = \{\hat{x}+\hat{y},-\hat{x}+\hat{y},-\hat{x}-\hat{y},\hat{x}-\hat{y}\}$ respectively. We note that slightly different definitions of Eq. 1 appear in the literature, in that some definitions do not include the factor of $1/\sqrt{2}$. Caution must therefore be used before comparing directly the magnitude of pair-pair correlations in different references.

If superconducting order exists in the ground state, $P_{ij}$ reaches a constant value in the limit of large pair separations. Caution must be used in making predictions from small pair separations. When $i = j$, $P_{ij}$ reduces to a combination of charge and spin correlations; furthermore, when pairs at $i$ and $j$ share common lattice points spurious enhancement of pairing by $U$ can occur [S11][S7]. For this reason, we consider only pairs separated by more than two lattice spacings, and further average over $P_{ij}$ for all $|\vec{r}_{ij}| > 2$. This approach and a similar measure $\bar{P}$ of average long-range pairing has been used by several previous studies of pairing on finite lattices [S12][S13].

Another quantity that is often cited as evidence for Coulomb enhancement of superconducting pairing is the vertex contribution to the pair-pair correlations [S14]. The vertex contribution is the difference between $P_{ij}$ and the corresponding quantity calculated using the uncorrelated Greens function; a positive vertex contribution indicates an attraction between quasi-particles [S14]. It is important to point out however, that even if the vertex contribution is positive, Coulomb interactions may suppress pairing relative to the $U = 0$ limit—the vertex contribution is a necessary but not sufficient condition for superconductivity. The vertex contribution for $d_{x^2-y^2}$ pair-pair correlations is positive even for the $\rho = 1$ square lattice [S14], which is an antiferromagnetic insulator for finite $U$. The comparison of the bare $P_{ij}$ to its $U = 0$ value is a much more demanding criterion for the occurrence of correlation-enhanced SC. We require several criteria to determine at which densities pairing is enhanced by $U$:

- $\bar{P}(U)$ is greater than $\bar{P}(U = 0)$, or equivalently the ratio is greater than one. This enhancement should persist for moderate $U$ ($U \sim 4$). We find for each lattice we considered that only at specific densities $\rho \approx 0.5$ does this occur, with $\bar{P}(U)/\bar{P}(U = 0)$ reaching a smooth peak at $U \approx 4$. The enhancement of pairing should not be determined by the the single-particle level structure alone. For each lattice, we compared the calculated pair correlations with the pattern of single-particle gaps $\Delta$, defined hereafter as the one-electron energy difference between the highest occupied and the lowest unoccupied levels; we found no "global" correlation between gap size at a particular density and pairing enhancement. There is, however, a "local" correlation that determines whether the enhancement occurs for $\rho$ exactly 0.5 or for one of two neighboring closed shell configurations. This is discussed in Section S.4.

- We did find $\bar{P}(U)/\bar{P}(U = 0) > 1$ in several cases in the very small $\rho$ region ($\rho < 0.25$). We discount these cases because at small $\rho$ the pairing correlations were of very small magnitude, one order of magnitude or more weaker than for $\rho \sim 0.5$. Finite size effects are also worse in the case of only a few electrons, and for example in several cases (see below), $\bar{P}(U = 0)$ was identically zero for certain pairing symmetries in the small $\rho$ regime.

- As remarked in the main text, in the highly likely frustrated lattice with $t_{x+y} \lesssim t_x \approx t_y$ that the appropriate pair wavefunction should involve a sum over all nearest- and next-nearest neighbour sites. This is then a superposition of $d_{x^2-y^2}$ and $d_{xy}$ pairing. We have not attempted to determine the optimum superposition but instead report both $d_{xy}$ and $d_{x^2-y^2}$ results. Note that in all cases we found only suppression in the $s$ or $s_{xy}$ pairing symmetries.

### S.3.1. 4×4

Finite size effects are the most extreme in the 4×4 lattice (only five pair separations of distance $r > 2$ exist), but results here are exact. As shown in Fig.S1, at $U = 0$, $d_{x^2-y^2}$ pairing is strongest in the 4×4 lattice. For $d_{xy}$ pairing, $\bar{P}(U = 0)$ is identically zero for most $\rho$, so we have focused on only $d_{x^2-y^2}$ pair symmetry here. Fig. S1 compares the enhancement of $\bar{P}$ to the inverse of the single-particle gap (the gap at $\rho$ exactly 0.5 is zero). While $\rho = 0.375$ and $\rho = 0.625$ have identical $U = 0$ gaps, $\rho = 0.375$ shows enhanced pairing but $\rho = 0.625$ does not. Fig. S2 shows $\bar{P}$ versus $U$ for all densities. $\rho = 0.375$ shows an enhancement which peaks at about $U \approx 4$. $\rho = 0.875$ shows a small enhancement, but only by a very small amount and at small $U$. Clearly $\rho = 0.375$ behaves differently from all other densities in this lattice. We will remark on the pairing enhancement at $\rho$ away from 0.5 in Section S.4, where we present a combined discussion for all the lattices.

In Fig. S3 we show the effect of $V_{ij}$ on the enhancement of pairing. Here we take $V_x = V_y = V_{x+y} = V$ and keep the ratio $V/U$ constant. As shown in Fig. S3, the enhancement of pairing at $\rho = 0.375$ by interactions is slightly smaller than with $V = 0$, but is still present. We further find that pairing away from the enhanced density is suppressed by an increased amount when $V$ is nonzero.

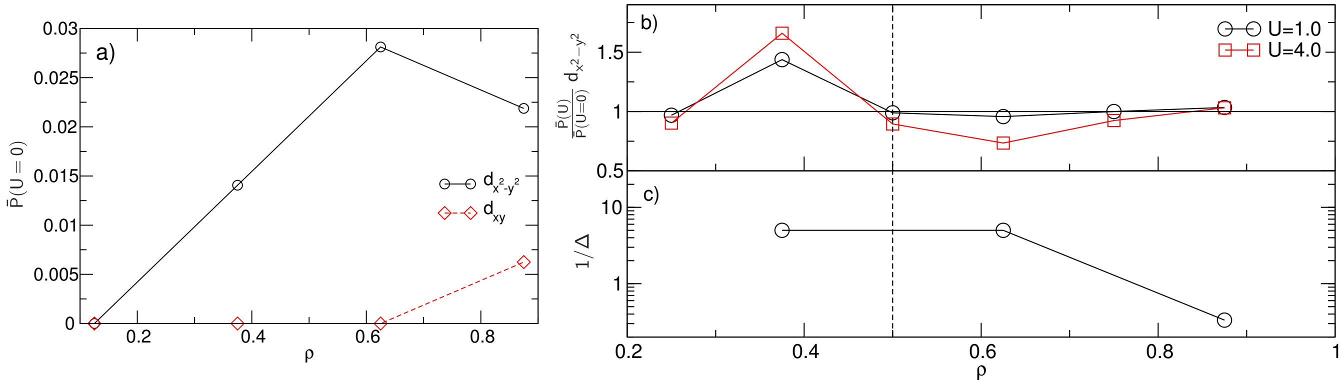


FIG. S1: Results for the 4×4 lattice with $t_x = 1$, $t_y = 0.9$, and $t_{x+y} = 0.8$. (a) $\bar{P}(U = 0)$ as a function of $\rho$. Circles are $d_{x^2-y^2}$ symmetry and diamonds are $d_{xy}$ symmetry. Only closed-shell densities are shown. (b) Exact $\bar{P}(U)/\bar{P}(U = 0)$ for $d_{x^2-y^2}$ pairing symmetry (c) Inverse of the single-particle gap $\Delta$ at $U = 0$.

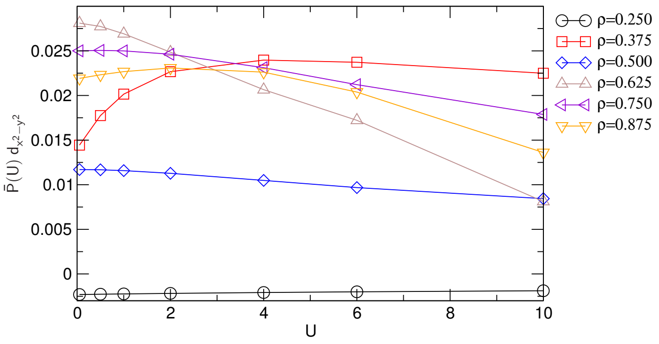


FIG. S2: 4×4 $\bar{P}(U)$ for $d_{x^2-y^2}$ pairing symmetry as a function of $U$. All parameters are the same as in Fig. S1.

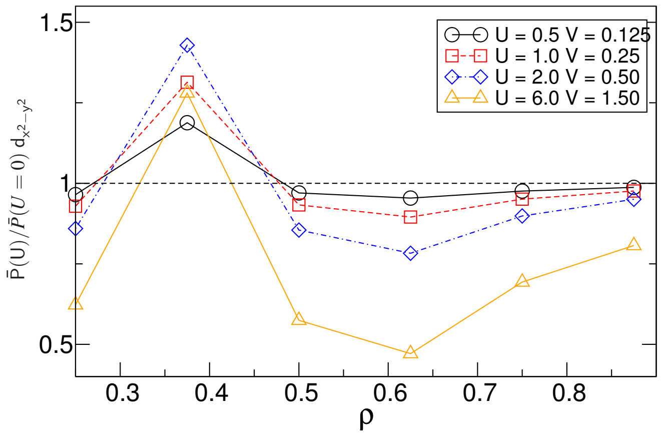


FIG. S3: 4×4 $\bar{P}(U)/\bar{P}(U=0)$ for $d_{x^2-y^2}$ pairing symmetry as a function of $U$ and $V$. All other parameters are the same as in Fig. S1.

### S.3.2. 6×6

As shown in Fig. S4, $d_{xy}$ pairing dominates in the 6×6 lattice for $0 < \rho < 1$. Coulomb enhancement of $d_{xy}$ pairing occurs at $\rho = 0.500$ (Fig. S4(b)) and enhancement of $d_{x^2-y^2}$ pairing at $\rho = 0.611$ (Fig. S5(a)). For small densities, the $d_{xy}$ $\bar{P}$ is identically zero at $U = 0$. For $\rho = 0.278$ $\bar{P}$ for $d_{xy}$ pairing does increase with $U$ (see Fig. S6), but has an extremely small value. Because of this and the finite-size effect giving zero pairing at $U = 0$ for this density, we do not believe this increase is significant. As shown in Fig. S6, at $\rho = 0.500$ $d_{xy}$ pairing as a function of $U$ shows a broad maximum at around $U \approx 4$, while the pairing for all other densities $\rho > 0.3$ is weakened by $U$. For $d_{x^2-y^2}$ pairing, there is a similar broad peak around $U \approx 3$ for $\rho = 0.611$ (Fig. S6); a small amount of enhancement at $\rho = 0.833$ is present for only very small $U$.

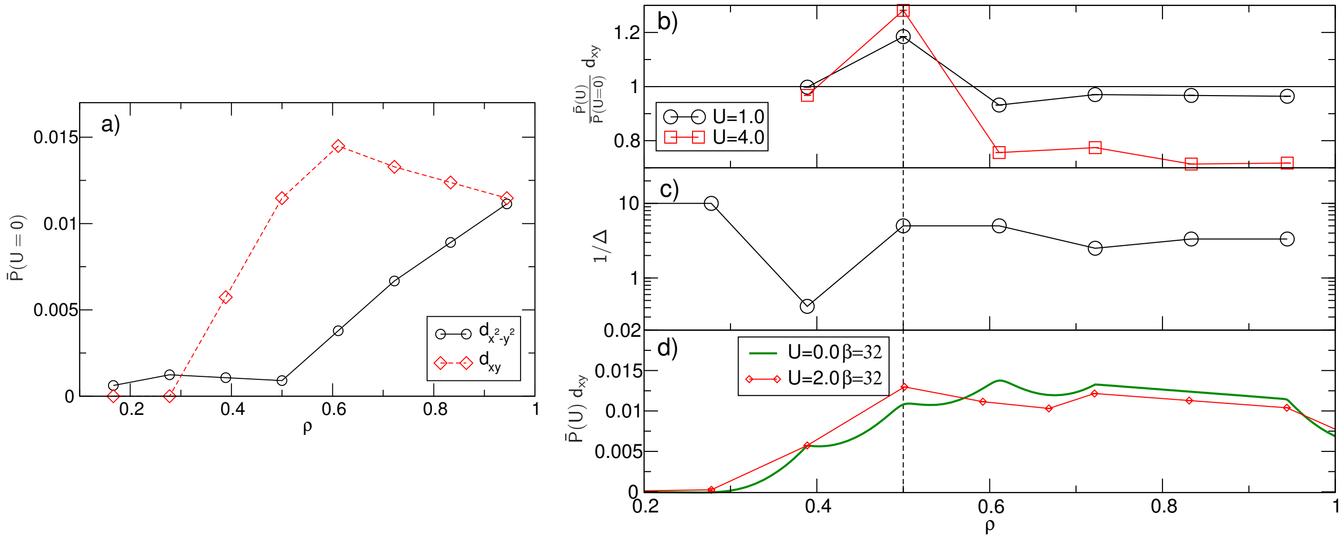


FIG. S4: Results for the 6×6 lattice with $t_x = 1$, $t_y = 0.9$, and $t_{x+y} = 0.8$. (a) $\bar{P}(U = 0)$ as a function of $\rho$. Circles are $d_{x^2-y^2}$ symmetry and diamonds are $d_{xy}$ symmetry. Only closed-shell densities are shown. (b) $\bar{P}(U)/\bar{P}(U = 0)$ calculated with PIRG for $d_{xy}$ pairing symmetry (c) Inverse of the single-particle gap $\Delta$ at $U = 0$ (d) $\bar{P}(U)$ from DQMC.

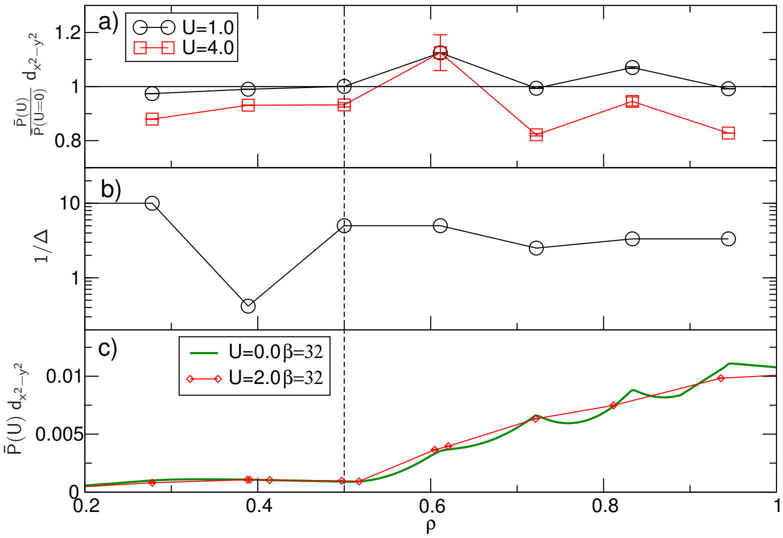


FIG. S5: Results for the 6×6 lattice with $t_x = 1$, $t_y = 0.9$, and $t_{x+y} = 0.8$ for $d_{x^2-y^2}$ pairing symmetry. (a) $\bar{P}(U)/\bar{P}(U = 0)$ calculated with PIRG (b) Inverse of the single-particle gap $\Delta$ at $U = 0$ (c) $\bar{P}(U)$ from DQMC. The dashed line indicates $\rho = 0.5$.

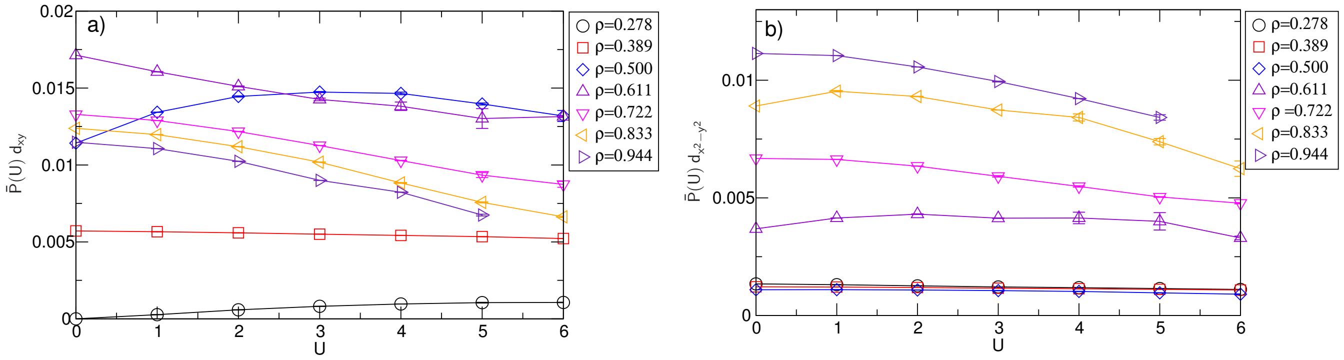


FIG. S6: 6×6 $\bar{P}(U)$ as a function of $U$ for all densities considered in Fig. S4 and Fig. S5. (a) $d_{xy}$ pairing symmetry. (b) $d_{x^2-y^2}$ pairing symmetry.

### S.3.3. 10×6

In the 10×6 lattice, $d_{xy}$ pairing also dominates (see Fig. S7) for most of the range $0 < \rho < 1$, although the difference is less than for the 6×6 lattice. Unlike the 6×6, here $d_{x^2-y^2}$ pairing is enhanced by $U$ at $\rho \sim 0.5$ (Fig. S8(a)) while $d_{xy}$ pairing is not enhanced significantly at any $\rho$ (Fig. S7(b)). As for 4×4 and 6×6, the enhancement at $\rho = 0.566$ appears to reach a maximum again around $U \approx 4$ (Fig. S9); for this lattice size we were not able to reach larger $U$ values with the PIRG method. Note the absence of an one-to-one global relationship between $\Delta$ and $\bar{P}(U)$ in Fig. S7.

In Fig. S10 we show a comparison between PIRG and CPMC for selected densities on the 10×6 lattice. Results from CPMC are nearly identical to PIRG for $U$ up to $U \approx 2$, or for small densities. For larger densities CPMC with the free-electron trial function tended to underestimate the pair-pair correlation function at large $U$.

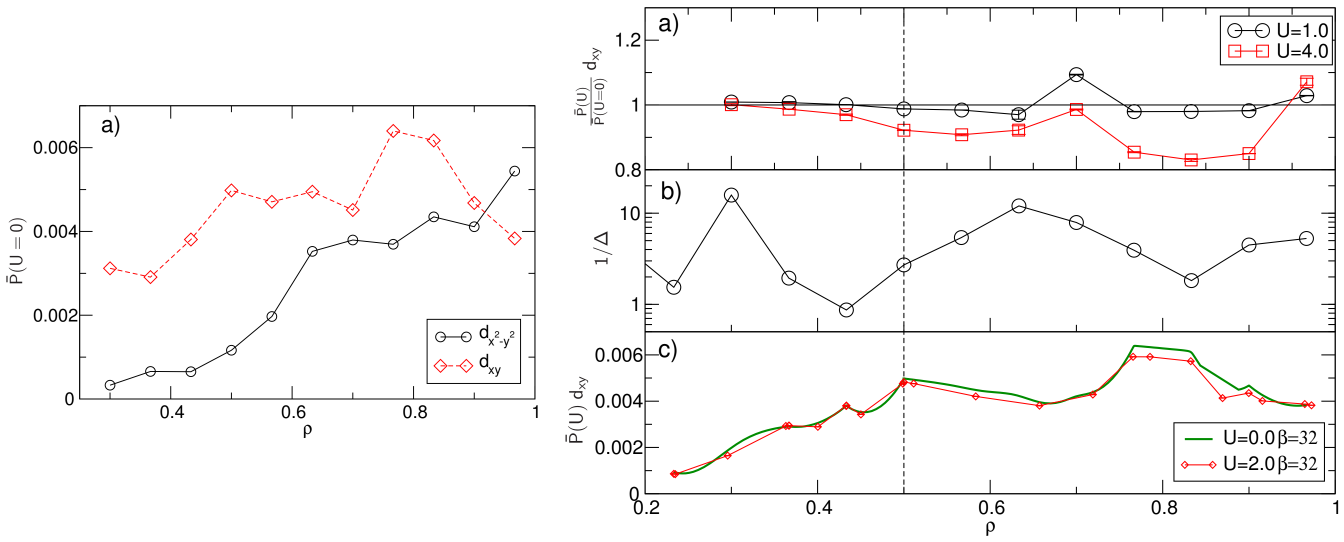


FIG. S7: Results for the 10×6 lattice with $t_x = t_y = 1$ and $t_{x+y} = 0.8$. Left: $\bar{P}(U=0)$ as a function of $\rho$. Circles are $d_{x^2-y^2}$ symmetry and diamonds are $d_{xy}$ symmetry. Only closed-shell densities are shown. Right: (a) $\bar{P}(U)/\bar{P}(U=0)$ for $d_{xy}$ pairing symmetry calculated with PIRG (b) Inverse of the single-particle gap $\Delta$ at $U = 0$ (c) $\bar{P}(U)$ for $d_{xy}$ symmetry from DQMC.

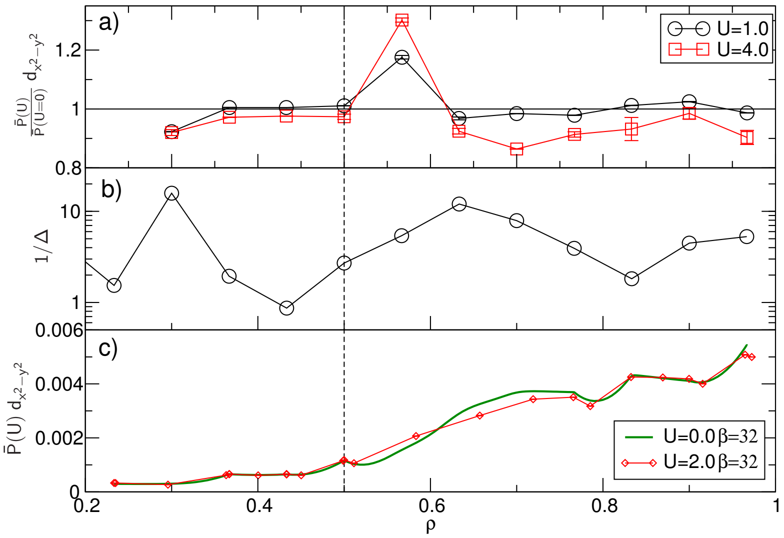


FIG. S8: Results for the 10×6 lattice with $t_x = t_y = 1$ and $t_{x+y} = 0.8$, for $d_{x^2-y^2}$ pairing symmetry as a function of $\rho$. (a) $\bar{P}(U)/\bar{P}(U=0)$ calculated with PIRG (b) Inverse of the single-particle gap $\Delta$ at $U = 0$ (c) $\bar{P}(U)$ from DQMC. The dashed line indicates $\rho = 0.5$.

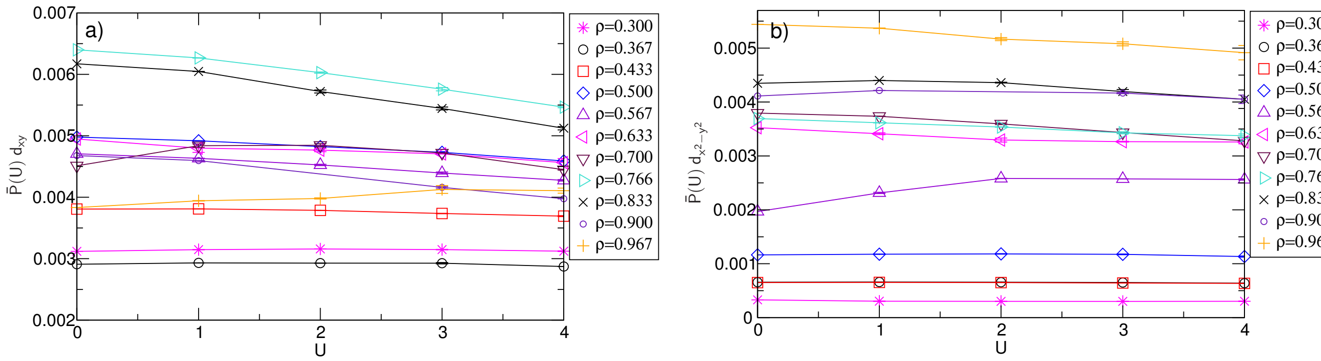


FIG. S9: 10×6 $\bar{P}(U)$ as a function of $U$ for all densities considered in Fig. S7 and Fig. S8. (a) $d_{xy}$ pairing symmetry (b) $d_{x^2-y^2}$ pairing symmetry.

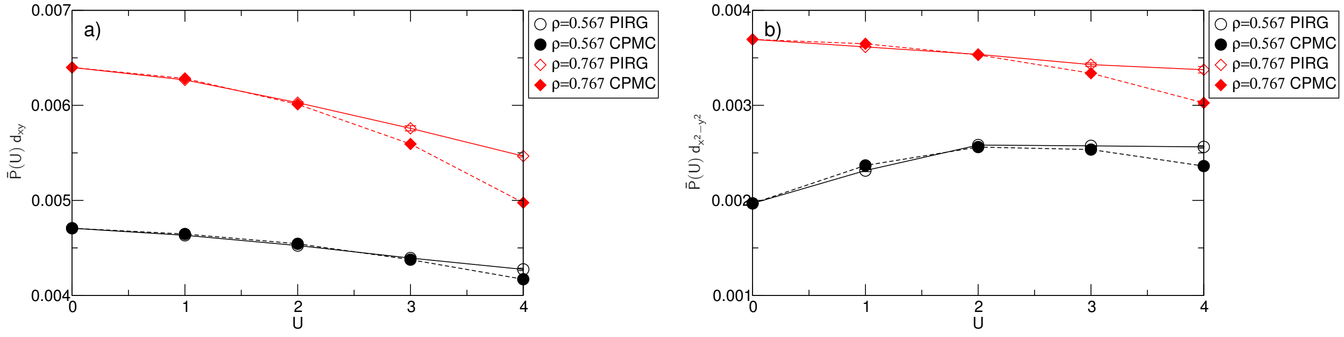


FIG. S10: Comparison of PIRG and CPMC for the 10×6 lattice at selected densities. (a) $d_{xy}$ pairing symmetry (b) $d_{x^2-y^2}$ pairing symmetry.

### S.3.4. 10×10

For the 10×10 lattice the PIRG method becomes too time consuming. Here we instead used CPMC with a free-electron trial wavefunction. Comparisons between CPMC and PIRG for the smaller lattices (see Fig. S10) showed that CPMC is quite accurate up to $U \sim 2$ but begins to show deviations from PIRG at around $U \sim 4$, especially for larger $\rho$. Hence we have only considered $U \sim 2$ for the 10×10 lattice.

For the 10×10 lattice, $d_{xy}$ pairing is again stronger (Fig. S11). As shown in Fig. S11, $d_{xy}$ pairing is enhanced at a single density in the range $0.2 < \rho < 1$. This density corresponds again to one of two next closed shell configurations immediately adjacent to $\rho = 0.5$ (46 electrons). The $d_{x^2-y^2}$ pairing also shows some enhancement with $U$, but the $U$ and $\rho$ dependence is somewhat more complicated (Fig. S12). However, discounting the very small $\rho$ region (where $\bar{P}(U=0)$ is extremely small as seen in Fig. S11(a)), the only $\rho$ that continues to show enhancement up to $U = 2$ is the density immediately above $\rho = 0.5$, viz., 0.54. Note again the absence of a global relationship between $\Delta$ and $\bar{P}(U)$ in Figs. S11 and S12.

Fig.S13 further shows the $U$ dependence of $\bar{P}$ for several selected densities. For the enhanced pairing near $\rho \approx 0.5$ (such as $\rho = 0.46$ in Fig. S13), we find that $\bar{P}$ continues to increase up to the maximum $U = 2$ we considered. This is consistent with the pairing enhancement peaking at $U \approx 4$ as found in the smaller lattices.

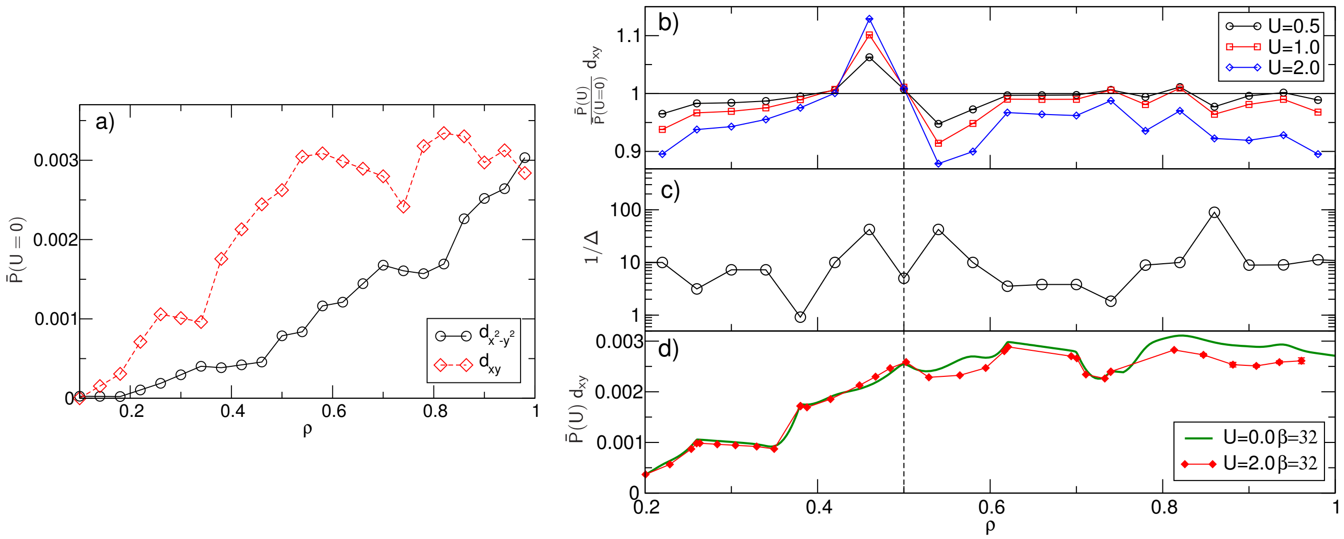


FIG. S11: Results for the 10×10 lattice with $t_x = 1$, $t_y = 0.9$, and $t_{x+y} = 0.8$. (a) $\bar{P}(U=0)$ as a function of $\rho$. Circles are $d_{x^2-y^2}$ symmetry and diamonds are $d_{xy}$ symmetry. Only closed-shell densities are shown. (b) $\bar{P}(U)/\bar{P}(U=0)$ for $d_{xy}$ pairing symmetry calculated from CPMC (b) Inverse of the single-particle gap $\Delta$ at $U = 0$ (c) $\bar{P}(U)$ for $d_{xy}$ pairing symmetry from DQMC. The dashed line indicates $\rho = 0.5$.

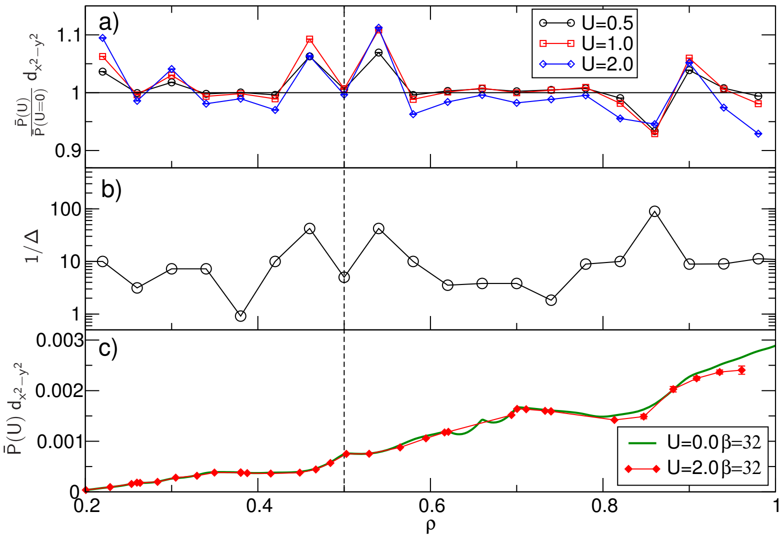


FIG. S12: Results for the 10×10 lattice with $t_x = 1$, $t_y = 0.9$, and $t_{x+y} = 0.8$, for $d_{x^2-y^2}$ pairing symmetry as a function of $\rho$. (a) $\bar{P}(U)/\bar{P}(U=0)$ calculated from CPMC (b) Inverse of the single-particle gap Δ at $U = 0$ (c) $\bar{P}(U)$ from DQMC. The dashed line indicates $\rho = 0.5$.

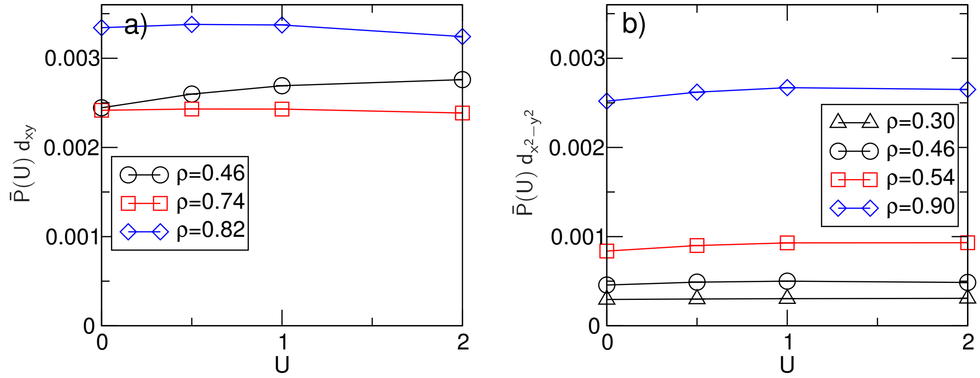


FIG. S13: 10×10 lattice (a) $\bar{P}(U)$ for $d_{xy}$ pairing symmetry as a function of $U$ for selected densities of Fig. S12. (b) $\bar{P}(U)$ for $d_{x^2-y^2}$ pairing symmetry as a function of $U$ for selected densities of Fig. S13.

## S.4. PAIRING ENHANCEMENT AWAY FROM $\rho$ EXACTLY 0.5

The pair binding energy in our calculations comes from the tendency to the Paired Electron Crystal (PEC), which is the strongest at $\rho = 0.5$. For number of carriers slightly deviating from precisely this density, the binding energy will still be nonzero, though weaker. In addition to nonzero binding energy, enhanced pair correlation requires pair mobility. In finite lattices, Δ is a measure of both one-particle and two-particle delocalization: the smaller the Δ, the greater the system mimics the thermodynamic limit and the greater is the delocalization. For enhanced pair correlations, the necessary requirements are then significant pair binding energy and relatively small $\Delta(\rho)$. Thus while $\Delta(\rho)$ does not have a global role in enhancing pair correlations (for $\rho$ far from 0.5 the pair binding energy is zero), it can have a "local" role, at and near $\rho = 0.5$. Based on this, it is now possible to understand all the results of Fig. 2 in the main paper.

In the 4×4 lattice, for $\rho = 0.5$ (8 electrons) the ground state is open shell for $U = 0$. Thus even though the $S = 0$ wavefunction has strong contributions from the short-bonded VB diagrams, in the absence of electron-phonon (e-p) interactions the actual ground state is in the $S = 1$ space. Thus the spin gap (SG), and hence the pair binding energy, are both negative here. This is why the enhanced pair correlation occurs for 6 electrons, where the binding energy is nonzero. The validity of this argument is easily proved, by repeating the calculations of Fig. 2 for parameters where for 8 electrons the $U = 0$ one-electron configuration is nondegenerate. This is true for $t_y \leq 0.4$ and $t_{x+y} = 0$. We show our computational results for this case in Fig. S14. Note that enhanced pair correlations now occur for $\rho$ exactly 0.5, which in this case has a smaller Δ than for $\rho = 0.375$.

In the 6×6 lattice we see from Fig. S4(b) that $\Delta(\rho)$ are the same for $\rho$ exactly 0.5 and for the closed-shell density immediately greater than this, while Δ is much larger for the density immediately smaller. Thus the larger binding energy at $\rho = 0.5$ dominates

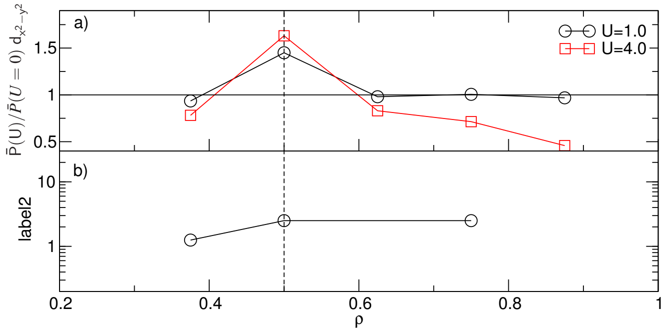


FIG. S14: (a) 4×4 $\bar{P}(U)/\bar{P}(U=0)$ for $d_{x^2-y^2}$ pairing symmetry, for $t_x = 1$, $t_y = 0.4$, and $t_{x+y} = 0$. (b) Inverse of the single-particle gap $\Delta$. For these parameters, enhancement occurs at $\rho = 0.500$.

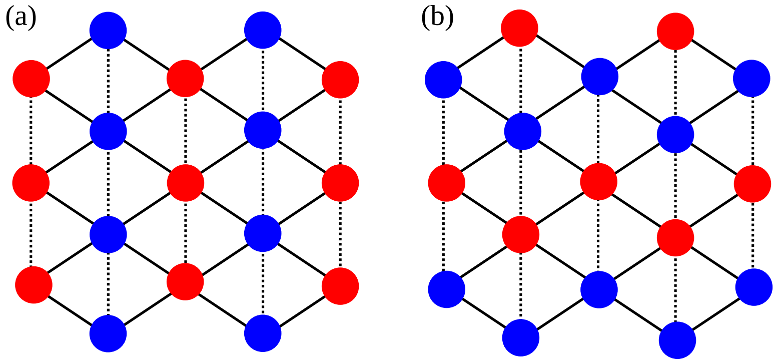


FIG. S15: The (a) Wigner crystal and the (b) PEC in the triangular lattice. Sites colored blue and red are charge-rich and charge-poor, respectively.

here.

For the 10×6 lattice, as seen from Fig. S6(c), $\Delta$ for $\rho$ immediately greater than 0.5 is smaller than $\Delta$ for $\rho$ exactly 0.5 by a factor of 2. Indeed, $\Delta(\rho = 0.5)$ for the 10×6 lattice is also twice as large as $\Delta(\rho = 0.5)$ for the 6×6 lattice. Pair mobility is therefore small and in spite of smaller binding energy, pair correlations are enhanced for $\rho$ larger than 0.5.

For the 10×10 lattice, $\Delta(\rho = 0.5)$ is again large: it is larger now by an order of magnitude compared to the two densities immediately next to 0.5. The enhancement therefore occurs to one of these densities (0.46) in the $d_{xy}$ channel and to both of them in the $d_{x^2-y^2}$ channel.

## S.5. THE PEC AND ITS OBSERVATION IN THE CHARGE TRANSFER SOLIDS (CTS).

We have previously studied $\rho = 0.5$ broken-symmetry insulating states in one-dimensional [S15–17], quasi-2D [S18,19], and 2D lattices [S20–22]. In these works we used the Peierls-extended Hubbard model,

$$H = H_K + H_U + H_V \tag{2}$$

$$H_K = -\sum_{\langle ij\rangle} t_{ij}[1+\alpha(a^\dagger_{ij}+a_{ij})]B_{i,j} + \omega_{SSH}\sum_{\langle ij\rangle} a^\dagger_{ij}a_{ij} + g\sum_j (b^\dagger_j + b_j)n_j + \omega_H \sum_j b^\dagger_j b_j \tag{3}$$

$$H_U = U\sum_i n_{i,\uparrow}n_{i,\downarrow} \qquad H_V = \frac{1}{2}\sum_{\langle ij\rangle} V_{ij}n_i n_j \tag{4}$$

where we have separated out the the kinetic energy and electron-phonon (e-p) interactions in Eq. 3 from the onsite and nearest neighbor (n.n.) electron-electron (e-e) interactions in Eq. 4. In Eq. 4 $\langle..\rangle$ imply n.n., $B_{i,j} = \sum_\sigma (c^\dagger_{i,\sigma}c_{j,\sigma} + H.c)$ and $t_{ij} = \{t_x, t_y, t_{x+y}\}$ on the frustrated 2D lattice. $V_{ij}$ can similarly have three components. $a^\dagger_{ij}$ creates a phonon on this bond, assumed to be dispersionless for simplicity [S17], with frequency $\omega_{SSH}$ and e-p coupling constant $\alpha$; $b^\dagger_j$ creates a Holstein intramolecular phonon on site $j$ with frequency $\omega_H$ and e-p coupling constant $g$.

In the semi-classical limit $\omega_{SSH} \to 0$, $\omega_H \to 0$, bond and charge distortions occur in the model in the limit of $\alpha = g = 0^+$.

Provided $V < V_c$, the charge order pattern found at $\rho = 0.5$ follows the pattern …1100… in 1D [S15,16]. Examples of these broken-symmetry states are shown in Fig. 1(b)-(e) of the paper. Both e-e and e-p interactions cooperatively reinforce the charge-spin-lattice order in the PEC.

The PEC is also found in 2D frustrated lattices [S21,22]. In the frustrated triangular lattice, if we assume $V_x \simeq V_y \simeq V_{x+y}$ there are two possible CO patterns that minimize e-e repulsion, as shown in Figs. S15(a) and S15(b). We refer to these as the linear and zigzag stripes, respectively [S20]. We ignore that there are three possible orientations of each stripe in the isotropic limit, as real CTS are far from this limit. In the limit $t_{ij} \to 0$ of the extended Hubbard model the linear and zigzag stripes are degenerate. There is, however, a fundamental difference between the two CO patterns. Denoting charge-rich and charge-poor sites as '1' and '0', respectively, the linear stripe has order …1111… in one of three directions in which the electron hopping is nonzero, and order …1010… in the two other directions. In contrast, the zigzag order has order …1100… in two of three directions and …1010… in the third direction. The linear stripe is thus the equivalent of the Wigner crystal within the triangular lattice, while the zigzag stripe is the PEC. Nonzero hopping stabilizes the zigzag stripe [S20] relative to the linear stripe, as any hopping in the latter creates either a double occupancy that costs energy $U$ or n.n. pairs that costs $V$. Further, due to the asymmetry in charge occupancy about any site within the zigzag structure, the bond-order between n.n. sites $i$ and $j$ $\langle c^\dagger_{i,\sigma} c_{j,\sigma} + H.c.\rangle$ is modulated within the PEC, which can imply spontaneous lattice distortion with nonzero e-p interactions, with the creation of spin singlets [S20]. In contrast, the Wigner crystal is likely to be AFM and gapless. Experimentally, either the charge density pattern if known, or the presence of SG is a signature that the CO is the PEC.

The CO patterns below the CO-SG transition in $\alpha$-(BEDT-TTF)$_2$I$_3$ (Fig. 2 in Reference S23), $\theta$-(BEDT-TTF)$_2$X (Fig. 7 in Reference S24), EtMe$_3$[Pd(dmit)$_2$]$_2$ (Fig. 3 in Reference S25) and $\beta$-(meso-DMBEDT-TTF)$_2$X (Fig. 2(b) in Reference S26) all show the charge periodicity expected in the PEC.

---


[S1] Z. G. Soos and S. Ramasesha. Valence-bond theory of linear Hubbard and Pariser-Parr-Pople models. *Phys. Rev. B*, 29:5410–5422, 1984.

[S2] S. Ramasesha and Z. G. Soos. Diagrammatic Valence-Bond Theory for Finite Model Hamiltonians. *Int. J. Quant. Chem.*, XXV:1003, 1984.

[S3] S. Ramasesha. A diagrammatic valence bond method for configuration interaction calculations in atoms and molecules. *Chem. Phys. Lett.*, 130:522, 1986.

[S4] T. Kashima and M. Imada. Path-integral renormalization group method for numerical study on ground states of strongly correlated electronic systems. *J. Phys. Soc. Jpn.*, 70:2287–2299, 2001.

[S5] T. Mizusaki and M. Imada. Quantum-number projection in the path-integral renormalization group method. *Phys. Rev. B*, 69:125110, 2004.

[S6] T. Yoshioka, A. Koga, and N. Kawakami. Mott transition in the Hubbard model on checkerboard lattice. *J. Phys. Soc. Jpn.*, 77:104702, 2008.

[S7] S. Dayal, R. T. Clay, and S. Mazumdar. Absence of long-range superconducting correlations in the frustrated $\frac{1}{2}$-filled band Hubbard model. *Phys. Rev. B*, 85:165141, 2012.

[S8] S. Zhang, J. Carlson, and J. E. Gubernatis. Constrained path Monte Carlo method for fermion ground states. *Phys. Rev. B*, 55:7464–7477, 1997.

[S9] R. Blankenbecler, D. J. Scalapino, and R. L. Sugar. Monte Carlo calculations of coupled boson-fermion systems. I. *Phys. Rev. D*, 24:2278, 1981.

[S10] E. Y. Loh and J. E. Gubernatis. Stable numerical simulations of models of interacting electrons in condensed-matter physics. In W. Hanke and Yu. V. Kopaev, editors, *Electronic Phase transitions*, pages 177–235. Elsevier, 1992.

[S11] R. T. Clay, H. Li, and S. Mazumdar. Absence of superconductivity in the half-filled band Hubbard model on the anisotropic triangular lattice. *Phys. Rev. Lett.*, 101:166403, 2008.

[S12] Z. B. Huang, H. Q. Lin, and J. E. Gubernatis. Quantum Monte Carlo study of spin, charge, and pairing correlations in the t-t$'$-$U$ Hubbard model. *Phys. Rev. B*, 64:205101, 2001.

[S13] T. Misawa and M. Imada. Origin of high-T$_c$ superconductivity in doped Hubbard models and their extensions: Roles of uniform charge fluctuations. *Phys. Rev. B*, 90:115137, 2014.

[S14] S. R. White, D. J. Scalapino, R. L. Sugar, N. E. Bickers, and R. T. Scalettar. Attractive and repulsive pairing interaction vertices for the two-dimensional Hubbard model. *Phys. Rev. B*, 39:R839–R842, 1989.

[S15] K. C. Ung, S. Mazumdar, and D. Toussaint. Metal-insulator and insulator-insulator transitions in the quarter-filled band organic conductors. *Phys. Rev. Lett.*, 73:2603–2606, 1994.

[S16] R. T. Clay, S. Mazumdar, and D. K. Campbell. The pattern of charge ordering in quasi-one dimensional organic charge-transfer solids. *Phys. Rev. B*, 67:115121, 2003.

[S17] R. T. Clay, R. P. Hardikar, and S. Mazumdar. Temperature-driven transition from the Wigner crystal to the bond-charge-density wave in the quasi-one-dimensional quarter-filled band. *Phys. Rev. B*, 76:205118, 2007.

[S18] R. T. Clay and S. Mazumdar. Co-operative bond-charge density wave and giant spin gap in the quarter-filled zigzag electron ladder. *Phys. Rev. Lett.*, 94:207206, 2005.

[S19] R. T. Clay, J. P. Song, S. Dayal, and S. Mazumdar. Ground state and finite temperature behavior of 1/4-filled band zigzag ladders. *J.*

*Phys. Soc. Jpn.*, 81:074707, 2012.

[S20] R. T. Clay, S. Mazumdar, and D. K. Campbell. Charge ordering in $\theta$-(BEDT-TTF)$_2$X materials. *J. Phys. Soc. Jpn.*, 71:1816–1819, 2002.

[S21] H. Li, R. T. Clay, and S. Mazumdar. The paired-electron crystal in the two-dimensional frustrated quarter-filled band. *J. Phys.: Condens. Matter*, 22:272201, 2010.

[S22] S. Dayal, R. T. Clay, H. Li, and S. Mazumdar. Paired electron crystal: Order from frustration in the quarter-filled band. *Phys. Rev. B*, 83:245106, 2011.

[S23] T. Ivek, B. Korin-Hamzic, O. Milat, S. Tomic, C. Clauss, N. Drichko, D. Schweitzer, and M. Dressel. Collective excitations in the charge-ordered phase of $\alpha$-(BEDT-TTF)$_2$I$_3$. *Phys. Rev. Lett.*, 104:206406, 2010.

[S24] M. Watanabe, Y. Noda, Y. Nogami, and H. Mori. Spin-Peierls transition in the charge-ordered organic conductor $\theta$-BEDT-TTF$_2$RbZn(SCN)$_4$. *J. Phys. Soc. Jpn.*, 76:124602, 2007.

[S25] M. Tamura, A. Nakao, and R. Kato. Frustration-induced valence-bond ordering in a new quantum triangular antiferromagnet based on [Pd(dmit)$_2$]. *J. Phys. Soc. Jpn.*, 75:093701, 2006.

[S26] T. Shikama et al. Magnetism and pressure-induced superconductivity of checkerboard-type charge-ordered molecular conductor $\beta$-(meso-DMBEDT-TTF)$_2$X (X = PF$_6$ and AsF$_6$). *Crystals*, 2:1502–1513, 2012.
